# Supplementary material for: Ab initio framework for nuclear scattering and reactions induced by light projectiles
Source: arXiv:2012.00228 source file (2020-12-01)
Supplement: Supplementary file 1 [file SupplementalMaterial.pdf]

# SUPPLEMENTAL MATERIAL FOR "AB INITIO FRAMEWORK FOR NUCLEAR SCATTERING AND REACTIONS INDUCED BY LIGHT PROJECTILES"

## Details of Slater determinant truncations and comparison with past approach in $n$-$\alpha$ scattering

The scattering of neutrons on $^4$He is a well established benchmark for ab initio methods in cluster dynamics and reaction theory. Here, we use $n$-$\alpha$ scattering to test the sensitivity of scattering observables to truncations in the many-body SD basis expansion of Eq. (3), as well as to demonstrate the equivalence of the present formalism and that of Ref. [28] at convergence in the HO expansion. For both tests we adopt the N$^3$LO NN interaction of Ref. [34], softened via a SRG transformation with resolution scale $\lambda_{\rm SRG} = 2.0$ fm$^{-1}$ in two-body space, denoted NN-only. The calculations are performed with an HO frequency of $\hbar\omega = 20$ MeV at $N_{\rm max} = 11$ and $N_{\rm max} = 15$.

TABLE I. Phase shifts for the $^2P_{3/2}$ channel of $n$+$\alpha$ scattering (in deg) at various center of mass energies. The parameter $t$ specifies the fixed truncation level before re-scaling with the channel norm.

| $E_{\rm CM}$ | $N_{\rm max} = 15$ | | | $N_{\rm max} = 11$ | | |
|---|---|---|---|---|---|---|
| (MeV) | $t = 10^{-5}$ | $t = 10^{-6}$ | $t = 10^{-7}$ | $t = 10^{-5}$ | $t = 10^{-6}$ | $t = 10^{-7}$ |
| 0.66 | 10.900 | 10.869 | 10.888 | 12.720 | 12.727 | 12.726 |
| 1.36 | 44.484 | 44.550 | 44.581 | 49.750 | 49.772 | 49.770 |
| 1.51 | 53.332 | 53.432 | 53.457 | 58.475 | 58.496 | 58.495 |
| 2.41 | 88.388 | 88.483 | 88.484 | 89.482 | 89.491 | 89.493 |
| 5.61 | 101.70 | 101.68 | 101.69 | 99.739 | 99.743 | 99.741 |
| 7.66 | 98.597 | 98.604 | 98.613 | 96.797 | 96.801 | 96.800 |
| 9.46 | 95.275 | 95.301 | 95.306 | 93.891 | 93.895 | 93.895 |

The total number of Slater determinants ($N_{\rm SD}$) in each reaction channel given by Eq. (3) can grow rapidly with $N_{\rm max}$ and with the number of nucleons in the system. However, a considerable number of such SD many-body states contributes only minimally to the wave function. Thus, it is advantageous to implement a truncation algorithm to make calculations computationally feasible. Given a fixed tolerance $t$, we remove from the expansion of Eq. (3) all Slater determinants with amplitude $|X_i| < t'$, where

$$t' = t\left[\sum_i^{N_{\rm SD}} X_i^2\right]^{1/2}.$$

That is, the full reaction channels are constructed and the SD expansion is subsequently truncated with a channel-dependent tolerance $t'$ so as to not disfavor Pauli-blocked channels that have small norms and for which most amplitudes $X_i$ are fairly small. Typically, the truncated reaction channel has a greater than 99.5% overlap with the original

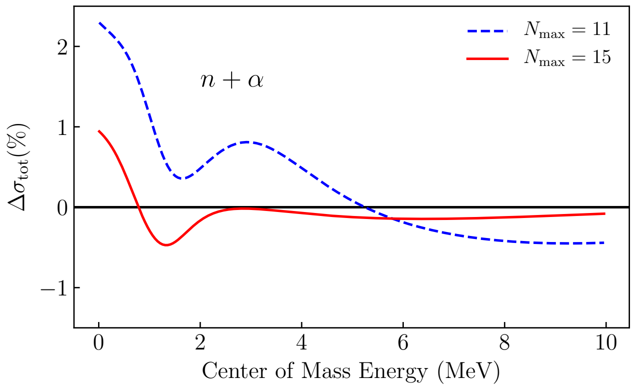


FIG. 1. The relative difference for the $n$-$\alpha$ cross section computed with the present approach and that of Ref. [28] is mostly at the subpercent level and decreases as convergence in $N_{\rm max}$ is reached.

one and a tolerance of $t = 10^{-5}$ is sufficient to reach an adequate convergence. As an example, the $n$-$\alpha$ scattering phase shifts in the $^2P_{3/2}$ partial wave over a wide energy range change by less than 0.1 deg when varying $t$ from $10^{-5}$ to $10^{-6}$ and $10^{-7}$ (Table I). In the present work we adopted a tolerance of $t = 2 \times 10^{-6}$ for $\alpha$-$\alpha$ scattering and $t = 10^{-6}$ for the $^{12}$Be system.

The present formalism and the original approach of Ref. [28] become equivalent at convergence in the HO expansion. For example, in the case of the total $n$-$\alpha$ elastic scattering cross section, the relative difference between original and present methodologies is mostly at the sub-percent level, with somewhat larger deviations at lower energy arising from a small shift of around 50 keV at $N_{\rm max} = 11$ and 3 keV at $N_{\rm max} = 15$ in the predicted resonance positions (Fig. 1).
